# Supplementary material for: Interaction Matters: An Evaluation Framework for Interactive Dialogue Assessment on English Second Language Conversations
Source: arXiv:2407.06479 source file (2025-02-04)
Supplement: Supplementary file 1 [file Annotation_Munnal_Final.pdf]

# Annotation Munnal for SLEDE Dataset

## 1. Introduction to the task

In your annotation, two types of dialogue tasks would be included in this study conducted by a pair-wise discussion by second language speaker participants. The first task is a storytelling task, in this part, two speakers will share some experience or what they want to deliver based on the instructions (e.g., *share some ideas on how you think of education in your life*). In the second task, two speakers need to solve a problem (e.g., *improve the experience of international students during their stay in Australia; and help to organize a welcome event*) through a joint discussion.

Dialogue of the two tasks were both transcribed into text and you are ready to annotate based on the text. **Videos will be provided if needed for correction of the text you are assigned.** Please notify the researcher, if you pick any misinformation in the transcriptions compared with the original recordings during your annotation.

## 2. Hierarchy sequence of the label

| Label name | Label level | Label tag | example |
|---|---|---|---|
| reference word | Token level labels | [RA] | SPK_1<br>OK, that's all.<br><br>SPK_2<br>That's all I think maybe we should switch from another park. |

| | | | |
|---|---|---|---|
| | | | SPK_1<br>OK, wait for her [RA]. |
| noun & verb collocation in proper form | | [NVC] | SPK_1<br>No accidents.<br><br>SPK_2<br>No accent. No, no. Like the the Beijing, Beijing accent. Yeah, that's that's the point. Yeah. So it's about the environment.<br><br>SPK_1<br>Yeah, I think that's right [NVC]. |
| code-switching for communicative purposes | | [CS] | SPK_1<br>How do think of the educational policy in China?<br><br>SPK_2<br>Hard to say, it depneds on different uh, **diqu (地区) [CS]** in China |
| negotiation of meaning (appropriate tense to show meaning) | | [NM] | SPK_1<br>How you plan your next stage after graduate?<br><br>SPK_2<br>I don't sure, maybe ask my presents whether they want to buy a house here or not. |

| | | | |
|---|---|---|---|
| | | | SPK_1<br>I' m going to see [NM] how my partner thinks. |
| tense choice to indicate interactive aims (politeness in talking/ social distance/ context variance) [TT] | | [TT] | SPK_1<br>May [TT] I start first in this one?<br><br>SPK_2<br>Ok. |
| routinized resources (projector construction) | | [RR] | SPK_1<br>How you going today[RR]?<br><br>SPK_2<br>Not bad. |
| subordinate clauses | | [RC] | SPK_1<br>Everyone mandatory course.<br><br>SPK_2<br>Yeah, yeah. It's a mandatory clause, so. So everyone needs to learn it. I think this is a pretty nice things to make [RC], make people like learn more things to have a big view for that. |
| backchannels | Utterance level labels | [BC] | SPK_2<br>That's all I think maybe we should switch from another park.<br><br>SPK_1 |

| | | | |
|---|---|---|---|
| | | | Oh [BC]<br><br>SPK_2<br>Wait for her. We can do it myself. Let's see what the what is in that spoiler spoiler problem-solving discussion. |
| question-based responses | | [QR] | SPK_2<br>Wait for her. We can do it myself. Let's see what the what is in that spoiler spoiler problem solving discussion. Instruction and at least. You need to with your partner and decide to. What solution to provide what kind of problem? Because she was solar problem together in this part. All we need to wait for right now, right?<br><br>SPK_1<br><br>Yes, yes [QR]. Actually I need to pause here. |
| formulaic responses | | [FR] | SPK_1<br><br>Good morning, I'm here to take in this task for Rena's study and<br><br>SPK_2 |

| | | | |
|---|---|---|---|
| | | | It' s nice to meet you here [FR]<br><br>SPK_1<br><br>same |
| collaborative finishes | | [CF] | SPK_2<br>No accent. No, no. Like the the Beijing, Beijing accent. Yeah, that's that's the point. Yeah. So it's about environment. It's. Yeah, I think that's right.<br><br>SPK_1<br>OK, that's all. [CF] |
| epistemic copulas | | [H1] | It seems [H1] to be a huge problem. |
| epistemic modals | | [H2] | It might [H2] be a huge problem. |
| adjectives/ adverbs expressing possibility | | [H3] | It is likely [H3] that this is a huge problem. |
| non-factive verb phrase structure | | [H4] | This is possibly [H4] a huge problem. |
| impersonal subject + non-factive verb + NP | | [H5] | These conclusions suggest a huge problem [H5]. |
| feedback in the next turn | | [FB] | SPK_1<br>A lot of people just don't know. A second language.<br><br>SPK_1<br>Ohh. [FB] |

| | | | |
|---|---|---|---|
| | | | SPK_2<br>Spanish.<br><br>SPK_1<br>Yes. [FB] |
| topic extension with clear new context (change to utterance level, but more information context depends ) | Dialogue level labels | [T1] | SPK_2<br>But you see that in China is all it was, like a lot of people just.<br><br>SPK_1<br>Everyone mandatory course.<br><br>SPK_2<br>Yeah, yeah. It's a mandatory course. So everyone needs to learn it. I think this is a pretty nice things to make, make people like learn more things to have a big view for that. And we can learn some beyond our own major studies in the uni. [T5] |
| topic extension under the previous direction | | [T2] | SPK_2<br>But you see that in China is all it was, like a lot of people just.<br><br>SPK_1<br>Everyone mandatory course.<br><br>SPK_2<br>Yeah, yeah. It's a mandatory course. So ev |

| | | | |
|---|---|---|---|
| | | | eryone needs to learn it. I think this is a pretty nice things to make, make people like learn more things to have a big view for that. [T4] |
| topic extension with the same content | | [T3] | SPK_2<br>But you see that in China is all it was, like a lot of people just.<br><br>SPK_1<br>Everyone mandatory course.<br><br>SPK_2<br>Yeah, yeah. It's a mandatory course. So everyone needs to learn it. [T3] |
| repeat and no topic extension | | [T4] | SPK_2<br>But you see that in China is all it was, like a lot of people just.<br><br>SPK_1<br>Everyone mandatory course.<br><br>SPK_2<br>yeah. yeah. It's a mandatory course. [T4] |
| no topic extension and stop the topic at this point | | [T5] | SPK_2<br>But you see that in China is all it was, like a lot of people just.<br><br>SPK_1 |

| | | | |
|---|---|---|---|
| | | | Everyone mandatory course.<br><br>SPK_2<br>Yeah, yeah. [T5] |
| conversation opening | | [CO1]<br>[CO2]<br>[CO3]<br>[CO4]<br>[CO5] | CO1: nice greeting and show a good understanding of conversation opening in social interactions.<br><br>CO2: sounded greeting and show a basic understanding of the social role.<br><br>CO3: general greeting and didn't demonstrate a good understanding of the social role.<br><br>CO4: basic greeting.<br><br>CO5: no opening just start the discussion immediately. |
| conversation closing | | [CC1]<br>[CC2]<br>[CC3]<br>[CC4]<br>[CC5] | CC1: detailed summarization and smooth transition to the closing of the conversation.<br><br>CC2: transit to the closing naturally, but without any summarization of the discussion.<br><br>CC3: transit to of the discussion. |

| | | | |
|---|---|---|---|
| | | | CC4: demonstrate a translation to the end of the conversation.<br><br>CC5: no closing, just stop the conversation. |
| overall tone choice: very formal | | [OT1] | I’ m very honoured to be here… |
| overall tone choice: quite formal and some expressions are not that formal | | [OT2] | I’ m more than happy to see you here today… |
| overall tone choice: relatively not formal, most expressions are quite informal | | [OT3] | Happy to meet with you… |
| overall tone choice:<br>quite informal, but some expressions are still formal | | [OT4] | You know, meeting with you is quite happy… |
| overall tone choice: very informal | | [OT5] | Hey, how’ s going, nice today… |

## 3. Label classifications and definitions

### 3.1 Token level

| Label Category | Aspect | Definition |
|---|---|---|
| Reference word | Word choice | A reference word, also known as a referential word or referent, is a linguistic term used to describe a word or e |

| | | |
|---|---|---|
| | | xpression in a sentence that refers to or stands in place of something else in the text. Reference words are used to avoid repetition and to link different parts of a text together by indicating what a subsequent word or phrase relates to. Reference words can take various forms, including pronouns, demonstratives, and other words that replace or point to nouns or noun phrases. |
| Noun & verb collocation in proper form | | Collocations are words or phrases that habitually occur together, forming a strong and natural linguistic association. In the case of noun-verb collocations, a particular noun is often paired with a particular verb due to convention, tradition, or linguistic patterns. These collocations contribute to the fluency, idiomaticity, and naturalness of language.<br><br>Examples of noun-verb collocations:<br><br>Make a decision: "I need to make a decision."<br>Take a shower: "I usually take a shower in the morning."<br>Catch a cold: "I hope I don't catch a cold."<br>Give a speech: "She gave an inspiring speech." |
| Code-switching for communicative purposes | | Code-switching for communicative purposes refers to the deliberate or subconscious a |

| | | |
|---|---|---|
| | | lternation between two or more languages or dialects within a single conversation or utterance by bilingual or multilingual speakers. This linguistic phenomenon is employed to fulfill specific communicative needs or functions, such as clarifying a point, expressing identity, signaling solidarity or distinction, accommodating to the listener's language preference, or conveying concepts and emotions more effectively in one language over another. Code-switching is not merely a random mixing of languages but a sophisticated communicative strategy that reflects the speaker's linguistic competence and cultural awareness, often used to navigate and negotiate the social and contextual dynamics of interaction. |
| Negotiation of meaning (appropriate tense to show meaning) | Contextual tense usage | Negotiation of meaning refers to the interactive process through which speakers of different linguistic backgrounds or competencies collaboratively work to understand each other's intentions, messages, and linguistic expressions when communication breakdowns occur. This involves the use of clarification requests, confirmation checks, comprehension checks, and paraphrasing, among other communicative strategies, to ensure mutual understanding is achieved. The negotiation of |

| | | |
|---|---|---|
| | | meaning is a fundamental aspect of second language acquisition and communicative language teaching, highlighting the dynamic nature of language use and the active role learners play in constructing meaning through interaction. |
| Tense choice to indicate interactive aims (politeness / social distance/ context) | | Tense choice to indicate interactive aims involves the strategic use of verb tenses by speakers to fulfill specific communicative goals or intentions within an interaction. This linguistic strategy encompasses the selection of present, past, future, or perfect tenses to convey nuances of time, mood, or aspect, directly influencing the interpretation and direction of the dialogue. Through careful tense selection, speakers can clarify the timing of events, express certainty or speculation about future occurrences, reflect on past experiences, or emphasize the continuity or completion of actions, all of which serve to enhance the clarity, persuasiveness, or relational dynamics of the communication. Tense choice, therefore, is not merely a grammatical decision but a deliberate tool employed by adept language users to navigate conversations and achieve specific interactive aims. |

| | | |
|---|---|---|
| routinized resources (projector construction) | Interactional grammatical device | Routinized resources refer to patterns, practices, or tools that have become standardized and regularly employed within specific contexts or activities. These resources are often developed through repeated use over time, leading to a level of automation or routine in their application. In organizational or social settings, routinized resources help in streamlining processes, reducing the need for decision-making about routine tasks, and ensuring consistency in actions and outcomes. They can include documented procedures, established workflows, habitual practices, or even common language and scripts used in interpersonal interactions. |
| subordinate clauses | | Subordinate clauses, also known as dependent clauses, are groups of words that contain a subject and a verb but do not express a complete thought and therefore cannot stand alone as a sentence. They function within a sentence by providing additional information to the main clause, to which they are connected by subordinating conjunctions (such as "because," "although," "when," "if") or relative pronouns (such as "who," "which," "that"). Subordinate clauses serve various roles in sentences, including acting as adjectives, adverbs, or nouns, and are essen |

| | | |
|---|---|---|
| | | tial for adding complexity, detail, and nuance to communication. Their use enables speakers and writers to articulate relationships of cause and effect, contrast, condition, time, and more, enriching the expressiveness and depth of language. |

## 4. Questions to note

4.1 Q: What if I find multiple labels in one sentence/phrase/ token?

A: Label them all, and put all labels in the required formats indicated in this table.

4.2 Q: How to decide the tone in this dialogue?

A: After reading the whole dialogue, if you feel it is hard to decide based on your experience in daily communication, you can find the original video in the folder and watch it to find more information.

4.3 Do I need to correct the wrong points in the dialogue (e.g., grammatical error? )

A: No you don't need to, if you find it hard to understand for a wrong point, you can refer to the original videos. Please keep the original content in the dialogue transcriptions.

**5.** Reference to consider when you start the annotate

5.1 http://compprag.christopherpotts.net/swda.html#tags

5.2 http://ling-blogs.bu.edu/lx390f16/classification/

5.3 https://aclanthology.org/D19-3021.pdf
