# Supplementary material for: Interaction Matters: An Evaluation Framework for Interactive Dialogue Assessment on English Second Language Conversations
Source: arXiv:2407.06479 source file (2025-02-04)
Supplement: Supplementary file 2 [file Appendix_Acl.pdf]

# Prompt design questinnaire

Thank you for participating in this research. This research project has been approved for coverage under the ethics of the University of Melbourne (Ethics ID: 2022-24988-32929-3). It aims to investigate how the language model predicts and labels the dialogues in live human communications, and to further evalute the dialogue quality via interactive metrics.

This survey is for designing the speaking prompts in this study.

This questionnaire consists of three parts. It will take about 3 minutes.

## Basic information

Your name (or preferred name)

Your age

Your gender

- Male
- Female
- Non-binary / third gender
- Prefer not to tell

Current education/ job status

- highschool
- undergraduate
- graduate (Master)
- graduate research (PhD)
- employed

Your email address

## Study abroad experience

Your home country:

- ○ China
- ○ Australia
- ○ [ ] Other country

How long have you stayed in Australia

- ○ less than 6 months
- ○ 6 months - 1 year
- ○ 1-2 year
- ○ 2-3 year
- ○ below 5 year
- ○ 5-10 year
- ○ over 10 year

Your first language

Besides your first language, what other languages have your learnt or can you speak?

Do you have any study abroad experience or stay abroad experience in English speaking countries?
If so, which country?

- Yes
- No

For how long have you spent your time as a study abroad student in English speaking country?

- less than 1 month
- 1-2 month
- 3-6 month
- 6-12 month
- 1- 2 year (12-24 month)
- 2-5 year (25-60 month)
- more than 5 years (61 month)

What other countries have you stayed for the purpose of study/ work?

For how long?

- 1-3 month
- 3-12 month
- over a year (12 month)

## Language proficiency

How easy is it for you to communicate in English? (English native speakers can ignore this question)

- Very easy, I can understand others and communicate in English **all the time**
- Mostly easy, I can use English well **in most cases**, but have trouble sometimes
- Sometimes easy, I can express myself and understand others **slightly more often** than not
- Sometimes difficult, I struggle to express myself and understand others slightly **more often than not**
- Mostly difficult, I struggle to express myself and understand others **most of the time** but occasionally I manage
- Very difficult, I struggle to express myself and understand others (nearly) **all the time**

How often do you use English

- rarely
- sometimes
- often
- always

How long do you use English in your communication everyday

- less than 1 hour
- 1 to 3 hour
- 3 to 5 hour
- above 5 hour

## Block 4

Please score the below topics according to your preference

| | 0 | 1 | 2 | 3 | 4 | 5 | 6 | 7 | 8 | 9 | 10 | Not Applicable | |
|---|---|---|---|---|---|---|---|---|---|---|---|---|---|
| plan the schedule of an end-of-semester party | | | | | | | | | | | | | |
| improve the living experience for international students | | | | | | | | | | | | | |

| | 0 | 1 | 2 | 3 | 4 | 5 | 6 | 7 | 8 | 9 | 10 | Not Applicable | |
|---|---|---|---|---|---|---|---|---|---|---|---|---|---|
| decide a schedule for a two hour group discussion | | | | | | | | | | | | | |
| select an elective subject in new semester | | | | | | | | | | | | | |
| decide on how to distribute work for a formal presentation within group members | | | | | | | | | | | | | |
| work out a solution for improving oral English in university communcations | | | | | | | | | | | | | |
| give two solutions for improving the learning experience in BLS learning and teaching mode | | | | | | | | | | | | | |
| plan a route for University of Melbourne Open-day tour for high shcool graduates | | | | | | | | | | | | | |

| | 0 | 1 | 2 | 3 | 4 | 5 | 6 | 7 | 8 | 9 | 10 | Not Applicable | |
|---|---|---|---|---|---|---|---|---|---|---|---|---|---|
| decide two subjects which you would recommed to newly commerenced students in your major | | | | | | | | | | | | | |
| provide two methods to help international students in adjusting local culture in Melbourne | | | | | | | | | | | | | |

What are the common topics you focus or interested in daily chat?

Powered by Qualtrics
