# Supplementary material for: Interaction Matters: An Evaluation Framework for Interactive Dialogue Assessment on English Second Language Conversations
Source: arXiv:2407.06479 source file (2025-02-04)
Supplement: Supplementary file 3 [file speaking_instruments.pdf]

# Notes on Participation:

- The study you are about to participate in consists of two speaking tasks. For each task, you will need to discuss the problem and work out a solution together. For example, if the instructions ask you to plan an event for movie night, it is important that you **make an effort** to complete the task as though you **actually** give a solution to the requirement.

- For each speaking task you will have some time to prepare, when you are ready, you can start to talk.

- All two tasks don’t have time limitation, you can speak **as long as you like.**

# Let’s know each other a little bit!

- Your name?
- Your major?
- How long have you stayed in Australia?

# Part One : Storytelling: Having a chat together

# Instructions:
# Speakers should chat in this part

- Talk about how you two think **COVID-19 impacted your life**, for example, you can talk about topics related to your study, working plan, shopping style or anything else.
- Speaker **A** will start the conversation first.
- **You should both contribute and engage in the conversation!**

# Now, switch your role:
# Chat about the topic below

- Talk about how you two think **education** influenced your life.
- Speaker **B** should start the conversation first.
- **You should both contribute in the conversation!**

# Part Two:
# Problem solving discussion

## Instructions:
## Speakers should solve a problem together  in this part.

**You have at least 20 minutes to discuss the problem with your partner and decide on what solutions to provide.**

**After your discussion, you have 5 minutes to tell Rena how you want to solve the issue.**

**PLUS: Always feel free to add any your own ideas.**

**You and your partner are going to discuss together to solve a problem.**

**The University are going to hold a face-to-face 1-hour welcome seminar for newly arrived international students in Melbourne, you need to work out a schedule and covered topics in this seminar.**

Here are some ideas:

- how to get most of lectures
- travel tips in Melbourne
- how to communicate with your classmates

**Always feel free to add any your own ideas.**

**You would have 3-5 minutes in the end to present your plan.**

Adopted from Micheal (2022)

**You and your partner are going to talk on how to improve the language exchange program at university.**

The University of Melbourne Academic Skills holds a language exchange program for students in all levels across the university. Due to the pandemic, this program was transferred to online, and the participation of this program is not good.

Now you and your partner need to give 3 suggestions on how to better improve this program during the post-pandemic stage.

# Thanks for your participation!
