# Supplementary material for: Interaction Matters: An Evaluation Framework for Interactive Dialogue Assessment on English Second Language Conversations
Source: arXiv:2407.06479 source file (2025-02-04)
Supplement: Supplementary file 5 [file Prompt_Final.pdf]

Your age

Your gender

- ☐ Male
- ☐ Female
- ☐ Non-binary / third gender
- ☐ Prefer not to tell

Current education/ job status

- ☐ highschool
- ☐ undergraduate
- ☐ graduate (Master)
- ☐ graduate research (PhD)
- ☐ employed

Your email address

## Study abroad experience

Your home country:

- ☐ China
- ☐ Australia
- ☐  Other country

How long have you stayed in Australia

- ☐ less than 6 months
- ☐ 6 months - 1 year
- ☐ 1-2 year
- ☐ 2-3 year
- ☐ below 5 year
- ☐ 5-10 year
- ☐ over 10 year

Your first language

Besides your first language, what other languages have you learnt or can you speak?

Do you have any study abroad experience or stay abroad experience in English speaking countries?

If so, which country?

☐  Yes

☐ No

For how long have you spent your time as a study abroad student in English speaking country?

- ☐ less than 1 month
- ☐ 1-2 month
- ☐ 3-6 month
- ☐ 6-12 month
- ☐ 1- 2 year (12-24 month)
- ☐ 2-5 year (25-60 month)
- ☐ more than 5 years (61 month)

What other countries have you stayed for the purpose of study/ work?

For how long?

- ☐ 1-3 month
- ☐ 3-12 month
- ☐ over a year (12 month)

## Language proficiency

How easy is it for you to communicate in English? (English native speakers can ignore this question)

- ☐ Very easy, I can understand others and communicate in English **all the time**
- ☐ Mostly easy, I can use English well **in most cases**, but have trouble sometimes
- ☐ Sometimes easy, I can express myself and understand others **slightly more often** than not
- ☐ Sometimes difficult, I struggle to express myself and understand others slightly **more often than not**
- ☐ Mostly difficult, I struggle to express myself and understand others **most of the time** but occasionally I manage
- ☐ Very difficult, I struggle to express myself and understand others (nearly) **all the time**

How often do you use English

- ☐ rarely
- ☐ sometimes
- ☐ often
- ☐ always

How long do you use English in your communication everyday

- ☐ less than 1 hour
- ☐ 1 to 3 hour
- ☐ 3 to 5 hour
- ☐ above 5 hour

Block 4

Please score the below topics according to your preference

012345678910

Not Applicable

plan the schedule of an end-of-semester party

improve the living experience for international students

Not Applicable

012345678910

decide a schedule for a two hour group discussion

select an elective subject in new semester

decide on how to distribute work for a formal presentation within group members

work out a solution for improving oral English in university communcations

give two solutions for improving the learning experience in BLS learning and teaching mode

plan a route for University of Melbourne Open-day tour for high shcool graduates

Not  
Applicable

012345678910

decide two  
subjects which  
you would  
recommmed to  
newly  
commerenced  
students in your  
major

☒☐

provide two  
methods to help  
international  
students in  
adjusting local  
culture in  
Melbourne

☒☐

What are the common topics you focus or interested in daily chat?

Powered by Qualtrics
