# Supplementary material for: Interaction Matters: An Evaluation Framework for Interactive Dialogue Assessment on English Second Language Conversations
Source: arXiv:2407.06479 source file (2025-02-04)
Supplement: Supplementary file 6 [file Prompt_Final_nourl.pdf]

Your age

Your gender

- ☐ Male
- ☐ Female
- ☐ Non-binary / third gender
- ☐ Prefer not to tell

Current education/ job status

- ☐ highschool
- ☐ undergraduate
- ☐ graduate (Master)
- ☐ graduate research (PhD)
- ☐ employed

Your email address

## Study abroad experience

Your home country:

- ☐ China
- ☐ Australia
- ☐  Other country

How long have you stayed in Australia

- ☐ less than 6 months
- ☐ 6 months - 1 year
- ☐ 1-2 year
- ☐ 2-3 year
- ☐ below 5 year
- ☐ 5-10 year
- ☐ over 10 year

Your first language

Besides your first language, what other languages have you learnt or can you speak?

Do you have any study abroad experience or stay abroad experience in English speaking countries?

If so, which country?

☐ Yes

☐ No

For how long have you spent your time as a study abroad student in English speaking country?

- ☐ less than 1 month
- ☐ 1-2 month
- ☐ 3-6 month
- ☐ 6-12 month
- ☐ 1- 2 year (12-24 month)
- ☐ 2-5 year (25-60 month)
- ☐ more than 5 years (61 month)

What other countries have you stayed for the purpose of study/ work?

For how long?

- ☐ 1-3 month
- ☐ 3-12 month
- ☐ over a year (12 month)

## Language proficiency

How easy is it for you to communicate in English? (English native speakers can ignore this question)

- ☐ Very easy, I can understand others and communicate in English **all the time**
- ☐ Mostly easy, I can use English well **in most cases**, but have trouble sometimes
- ☐ Sometimes easy, I can express myself and understand others **slightly more often** than not
- ☐ Sometimes difficult, I struggle to express myself and understand others slightly **more often than not**
- ☐ Mostly difficult, I struggle to express myself and understand others **most of the time** but occasionally I manage
- ☐ Very difficult, I struggle to express myself and understand others (nearly) **all the time**

How often do you use English

- ☐ rarely
- ☐ sometimes
- ☐ often
- ☐ always

How long do you use English in your communication everyday

- ☐ less than 1 hour
- ☐ 1 to 3 hour
- ☐ 3 to 5 hour
- ☐ above 5 hour

Block 4

Please score the below topics according to your preference

|                                                                   | 0                                | 1 | 2 | 3 | 4 | 5 | 6 | 7 | 8 | 9 | 10 | Not<br>Applicable        |                      |
|-------------------------------------------------------------------|----------------------------------|---|---|---|---|---|---|---|---|---|----|--------------------------|----------------------|
| plan the<br>schedule of an<br>end-of-<br>semester party           | <input checked="" type="radio"/> |   |   |   |   |   |   |   |   |   |    | <input type="checkbox"/> | <input type="text"/> |
| improve the<br>living experience<br>for international<br>students | <input checked="" type="radio"/> |   |   |   |   |   |   |   |   |   |    | <input type="checkbox"/> | <input type="text"/> |

Not  
Applicable

0 1 2 3 4 5 6 7 8 9 10

decide a  
schedule for a  
two hour group  
discussion

☐☐

select an  
elective subject  
in new semester

☐☐

decide on how  
to distribute  
work for a formal  
presentation  
within group  
members

☐☐

work out a  
solution for  
improving oral  
English in  
university  
communcations

☐☐

give two  
solutions for  
improving the  
learning  
experience in BLS  
learning and  
teaching mode

☐☐

plan a route for  
University of  
Melbourne  
Open-day tour  
for high shcool  
graduates

☐☐

Not  
Applicable

0 1 2 3 4 5 6 7 8 9 10

decide two  
subjects which  
you would  
recommned to  
newly  
commerenced  
students in your  
major

☐☐

provide two  
methods to help  
international  
students in  
adjusting local  
culture in  
Melbourne

☐☐

What are the common topics you focus or interested in daily chat?
